# Supplementary material for: Measurement of final-state correlations in neutrino muon-proton mesonless production on hydrocarbon at $\langle E_\nu\rangle=3$ GeV
Source: arXiv:1805.05486 ancillary file (2018-09-18)
Supplement: Supplementary file 1 [file SupplementalMaterial1.pdf]

In Supplemental Material 1 the model-data comparisons are shown for single particle kinematics, the transverse kinematics imbalance $\delta p_{\mathrm{T}}$, and $\delta\phi_{\mathrm{T}}$ (for definition see Phys. Rev. C 94, 015503). The correlation matrices for the total uncertainty and the uncertainties from individual sources are also presented.

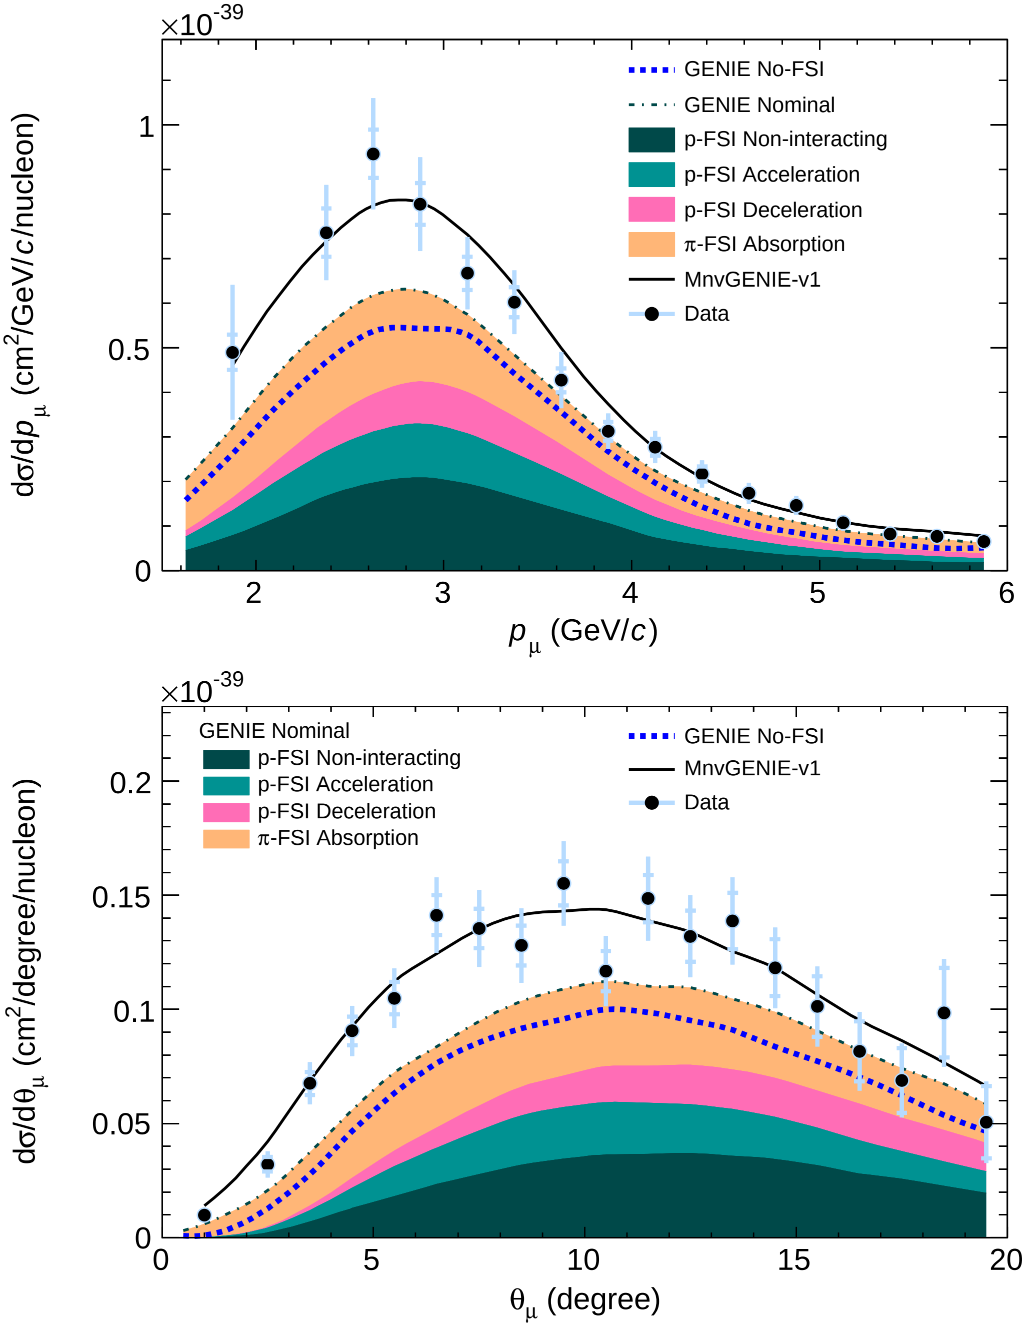


Figure 1: Differential cross sections in muon momentum $p_\mu$ (*up*) and polar angle $\theta_\mu$ (*low*) compared to GENIE predictions. MnvGENIE-v1 predictions describe the data within 1-$\sigma$ total uncertainty. The predicted shape is consistent among all models.

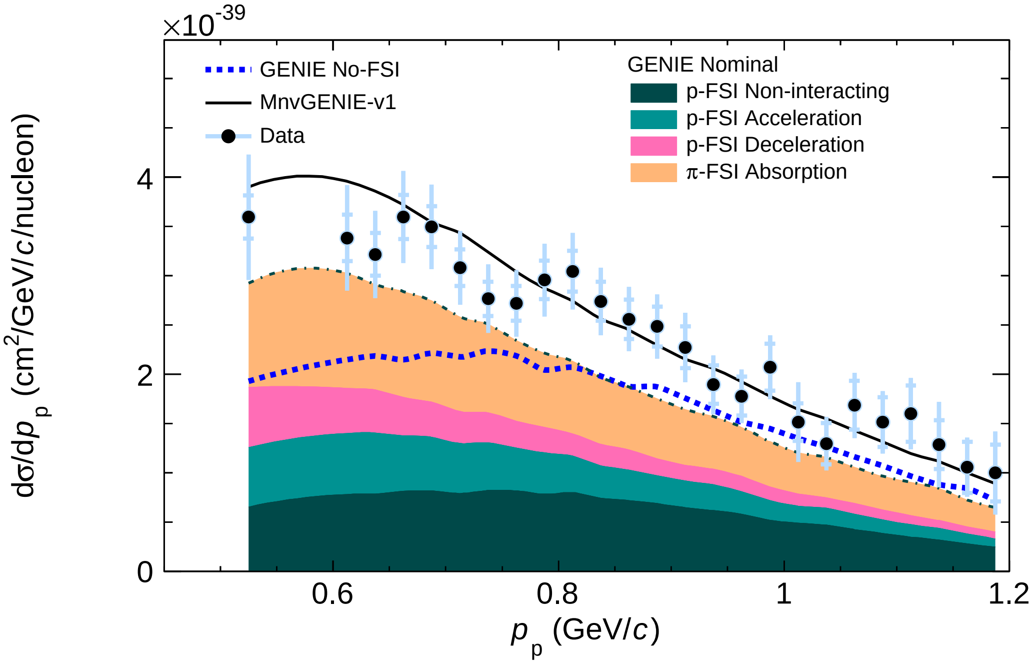


Figure 2: Differential cross section in proton momentum $p_{\mathrm{p}}$ compared to GENIE predictions. MnvGENIE-v1 predictions describe the data within 1-$\sigma$ total uncertainty.

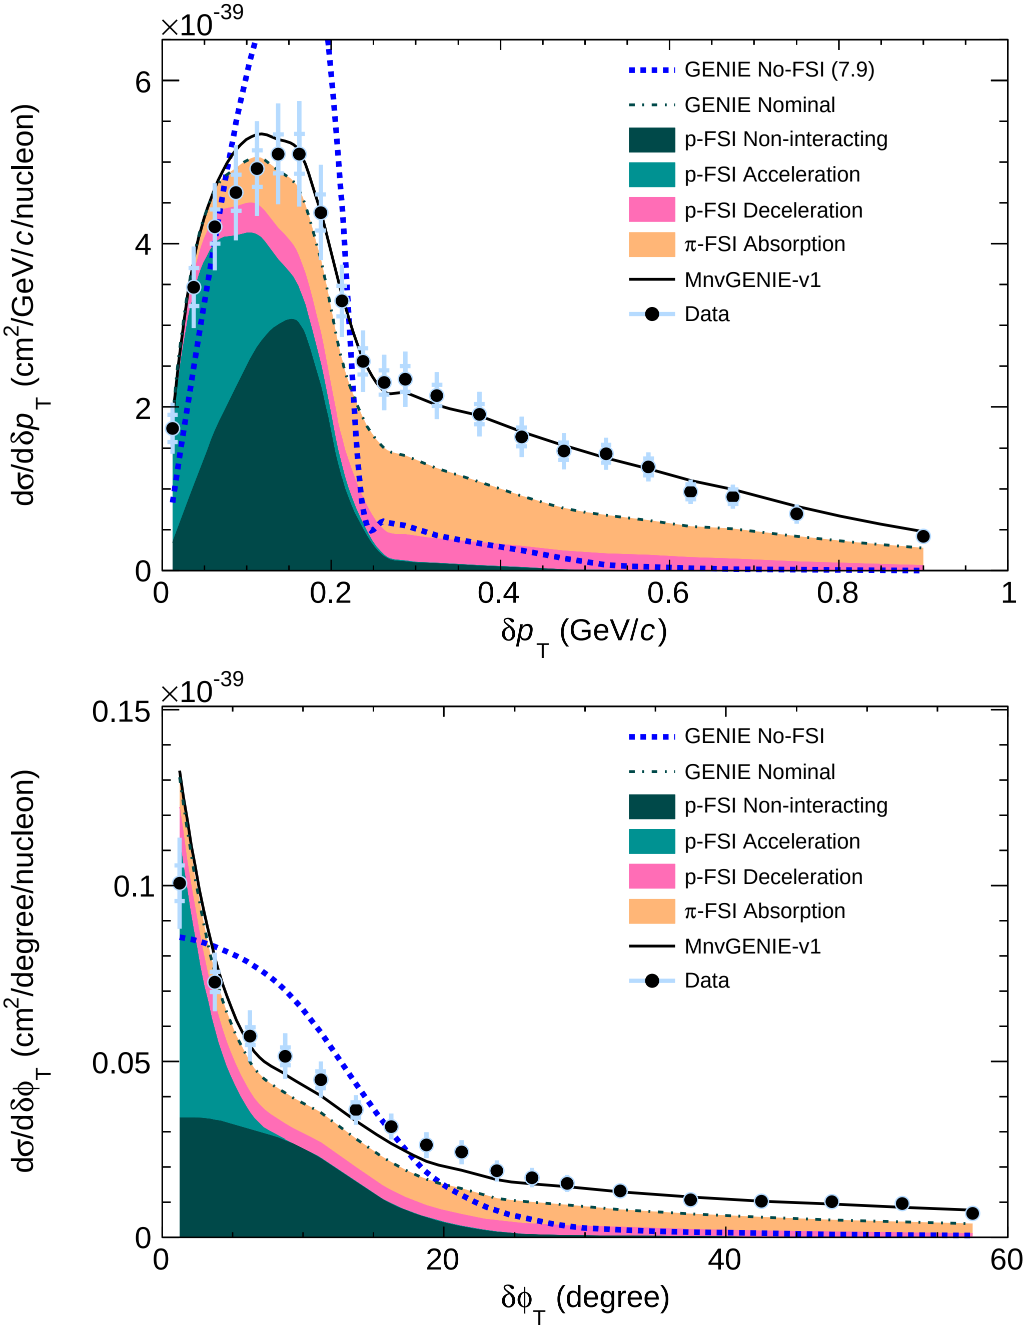


Figure 3: Differential cross section in transverse momentum imbalance $\delta p_{\mathrm{T}}$ and $\delta\phi_{\mathrm{T}}$ compared to GENIE predictions.

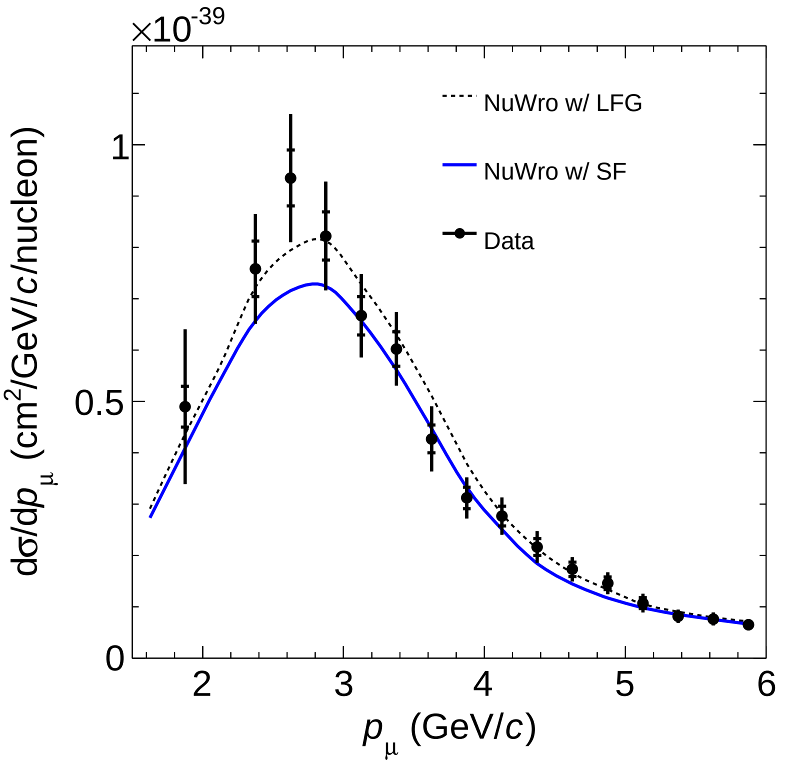


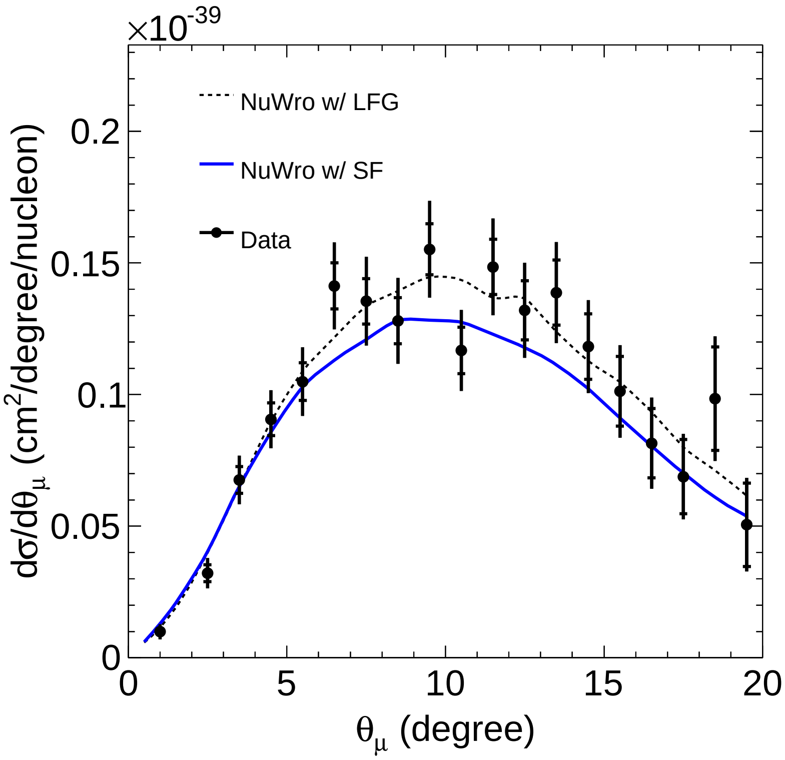


Figure 4: Differential cross sections in muon kinematics compared to NuWro predictions. NuWro predictions with SF describe the data within 1-$\sigma$ total uncertainty.

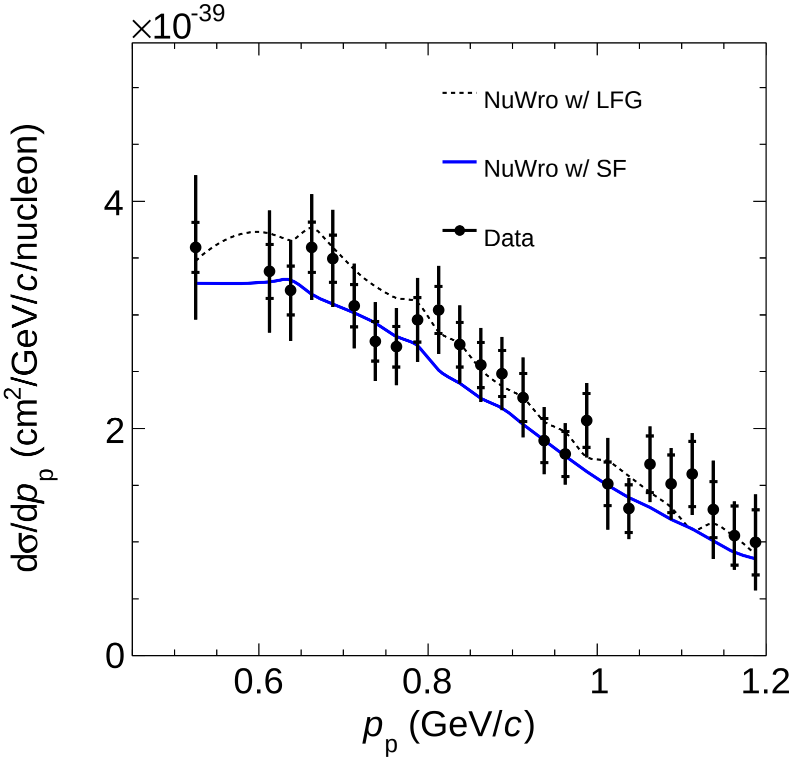


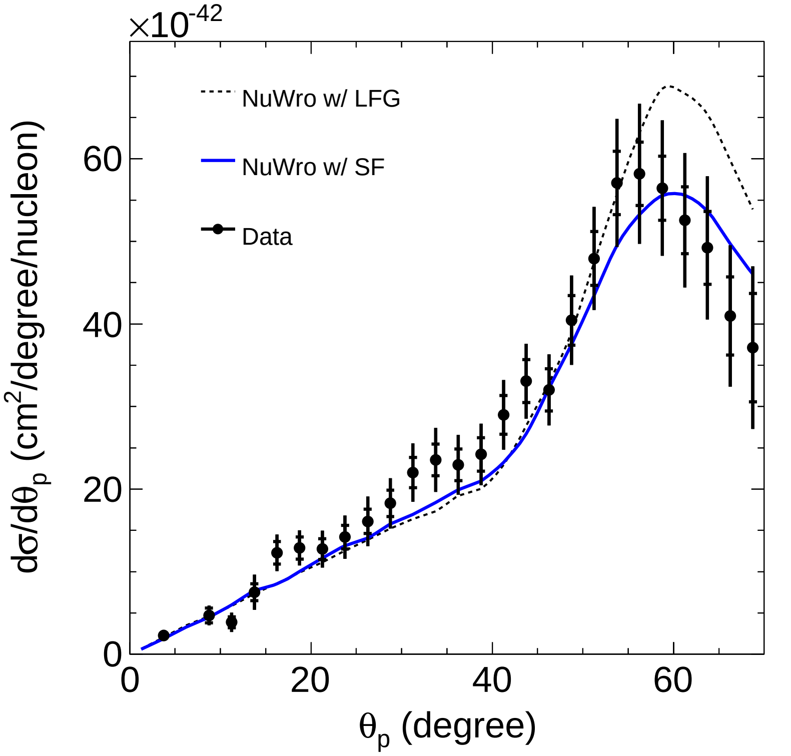


Figure 5: Differential cross sections in proton kinematics compared to NuWro predictions. NuWro predictions with SF describe the data within 1-$\sigma$ total uncertainty.

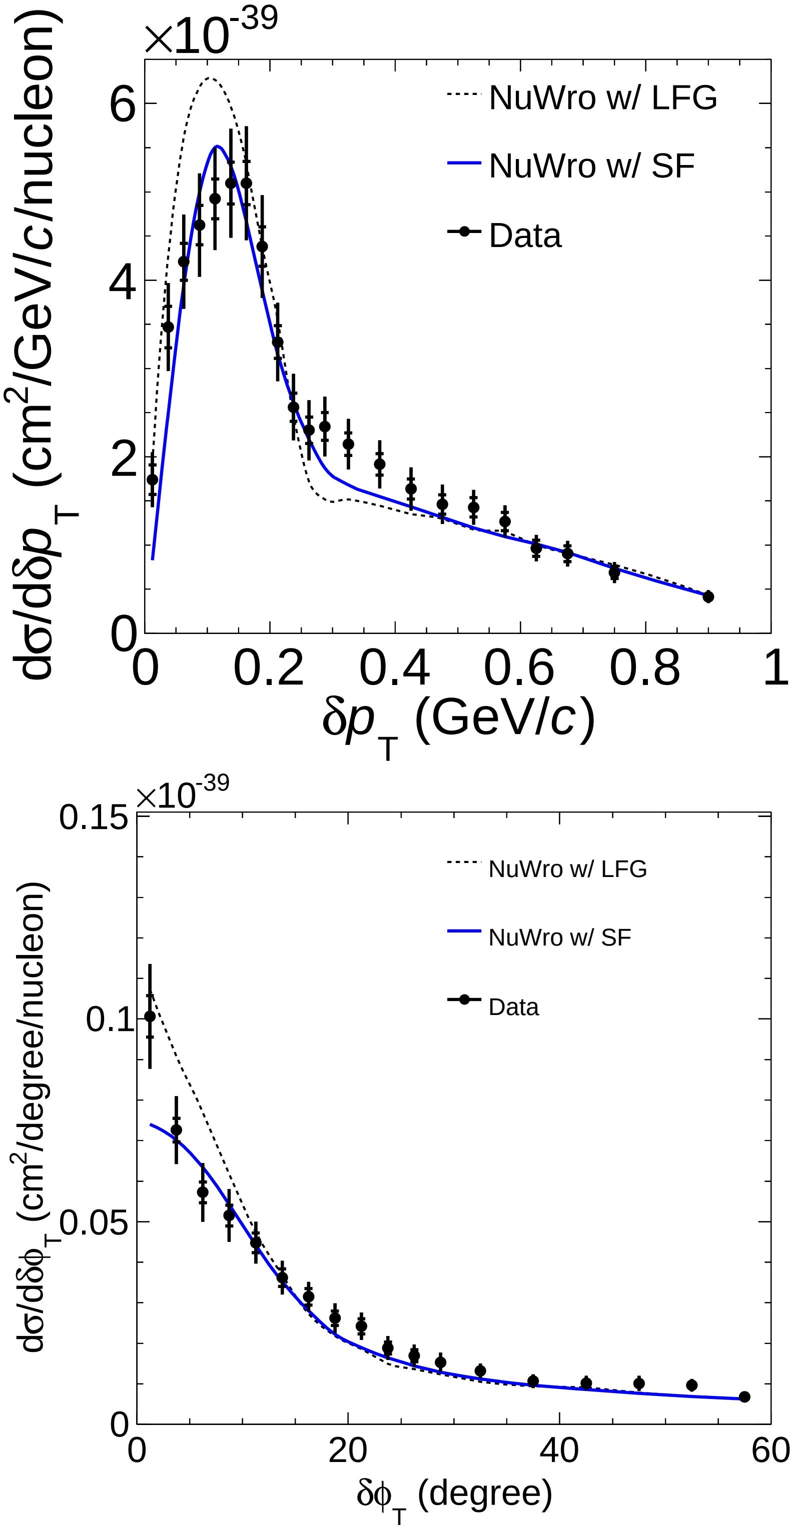


Figure 6: Differential cross section in transverse momentum imbalance $\delta p_{\mathrm{T}}$ and $\delta \phi_{\mathrm{T}}$ compared to NuWro predictions. NuWro predictions with SF has a deficit significantly in $\delta p_{\mathrm{T}}$ beyond 1-$\sigma$ total uncertainty.

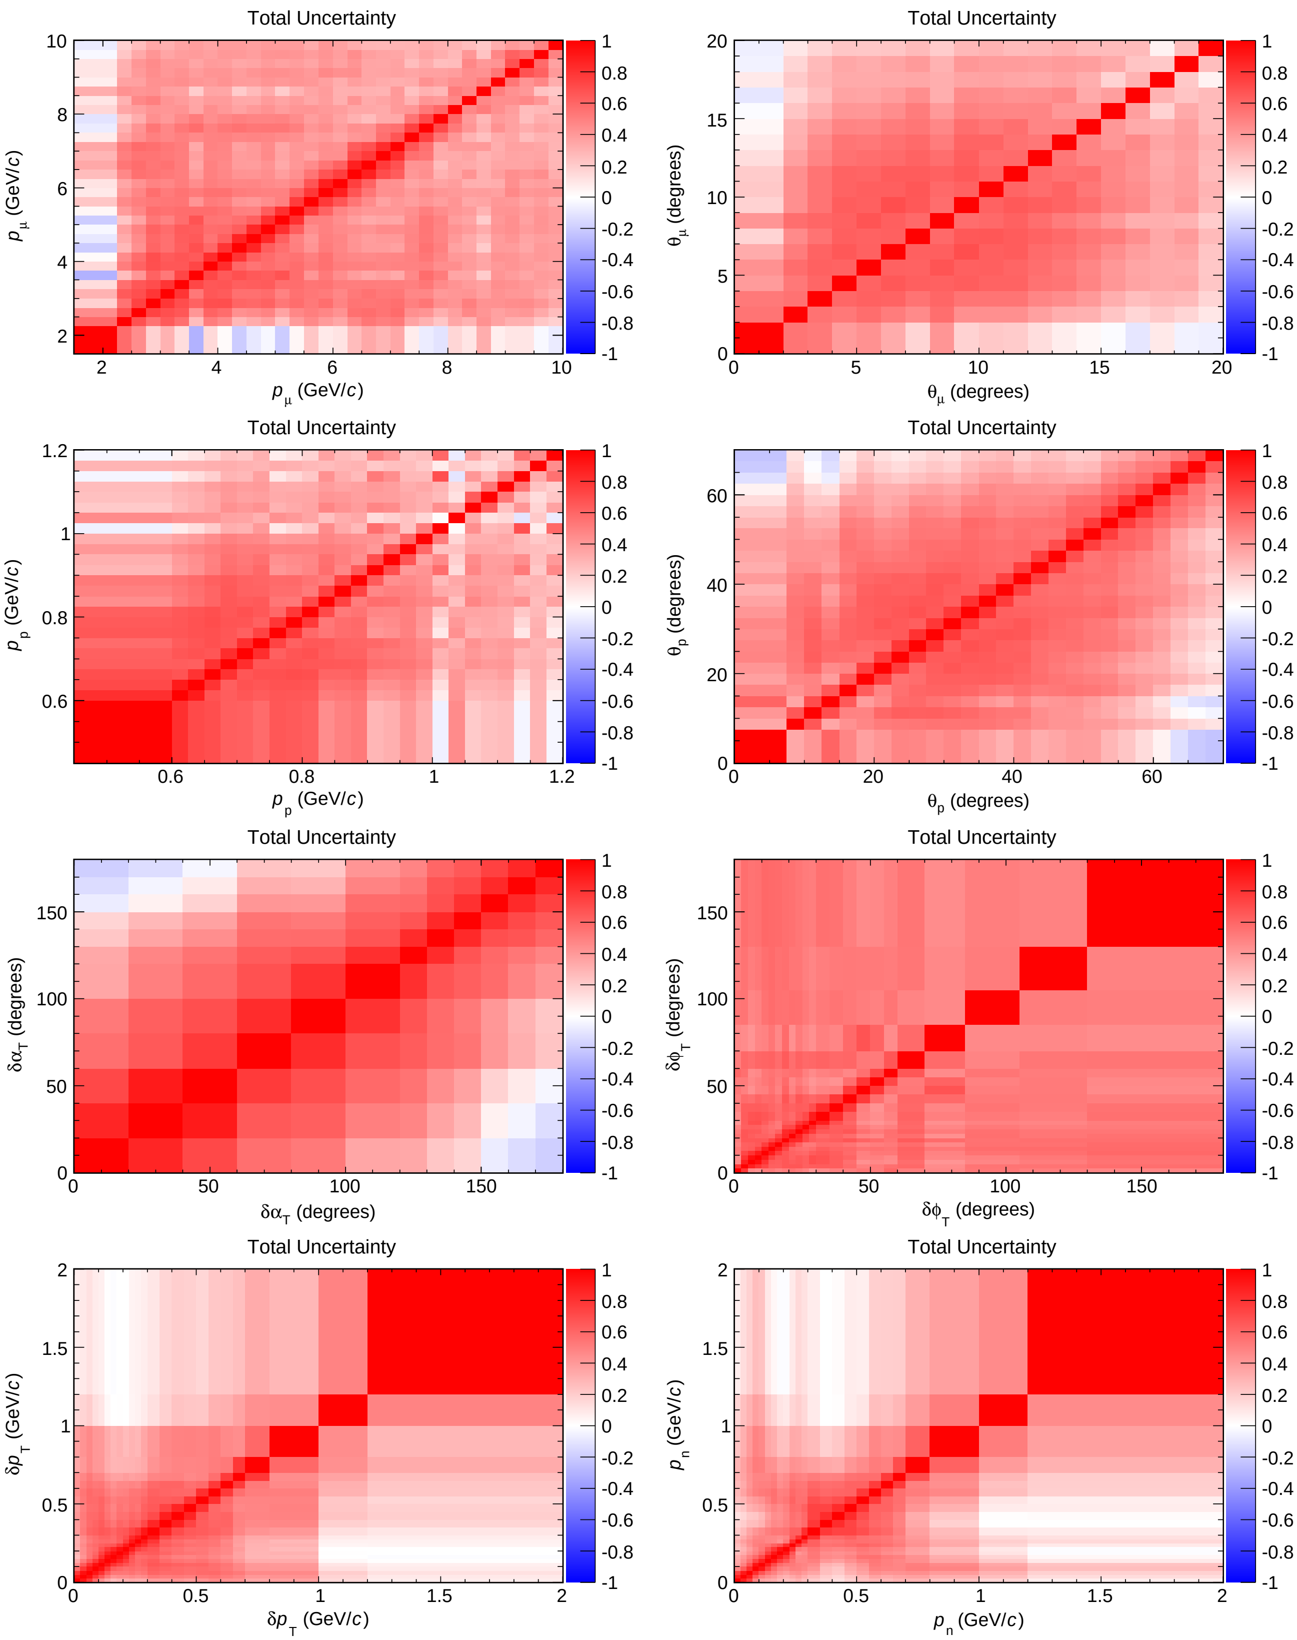


Figure 7: Total uncertainty correlation matrix for all variables.

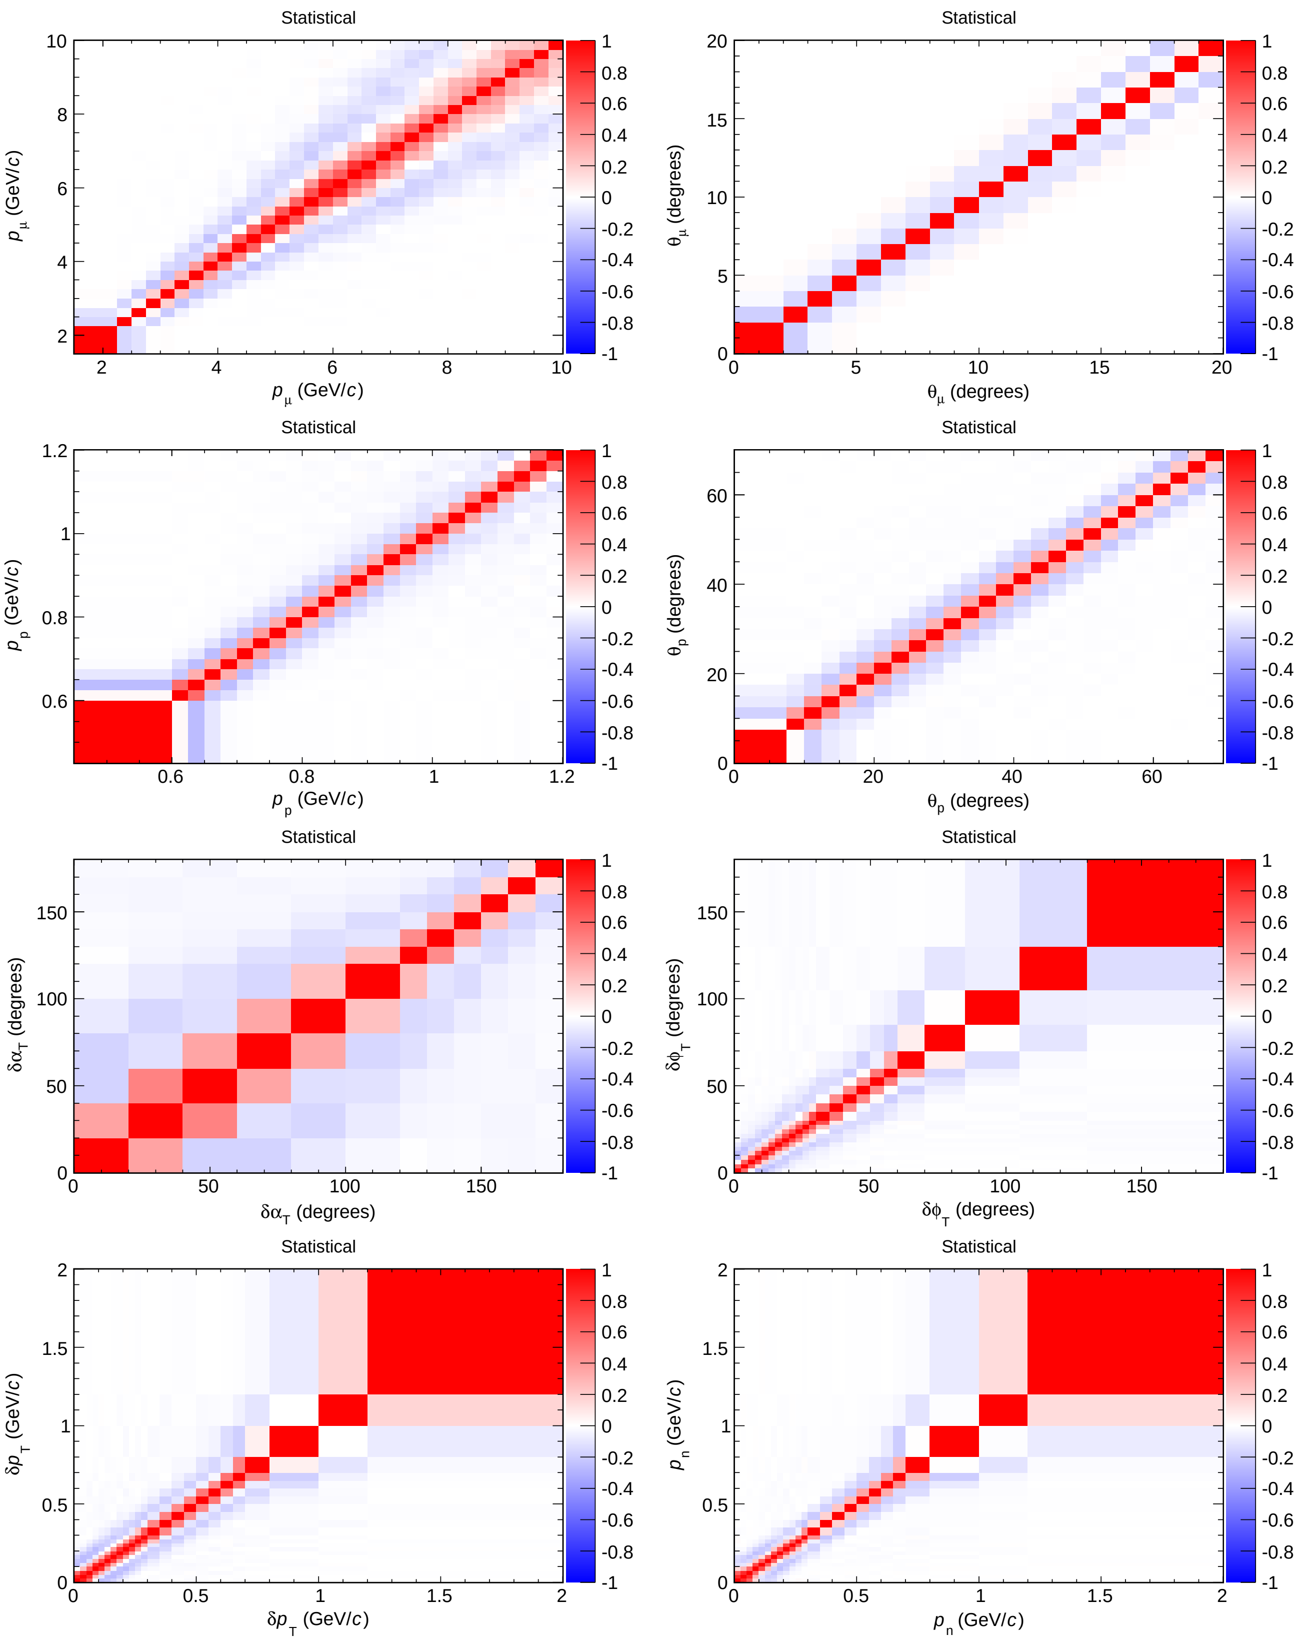


Figure 8: Statistical uncertainty correlation matrix for all variables.

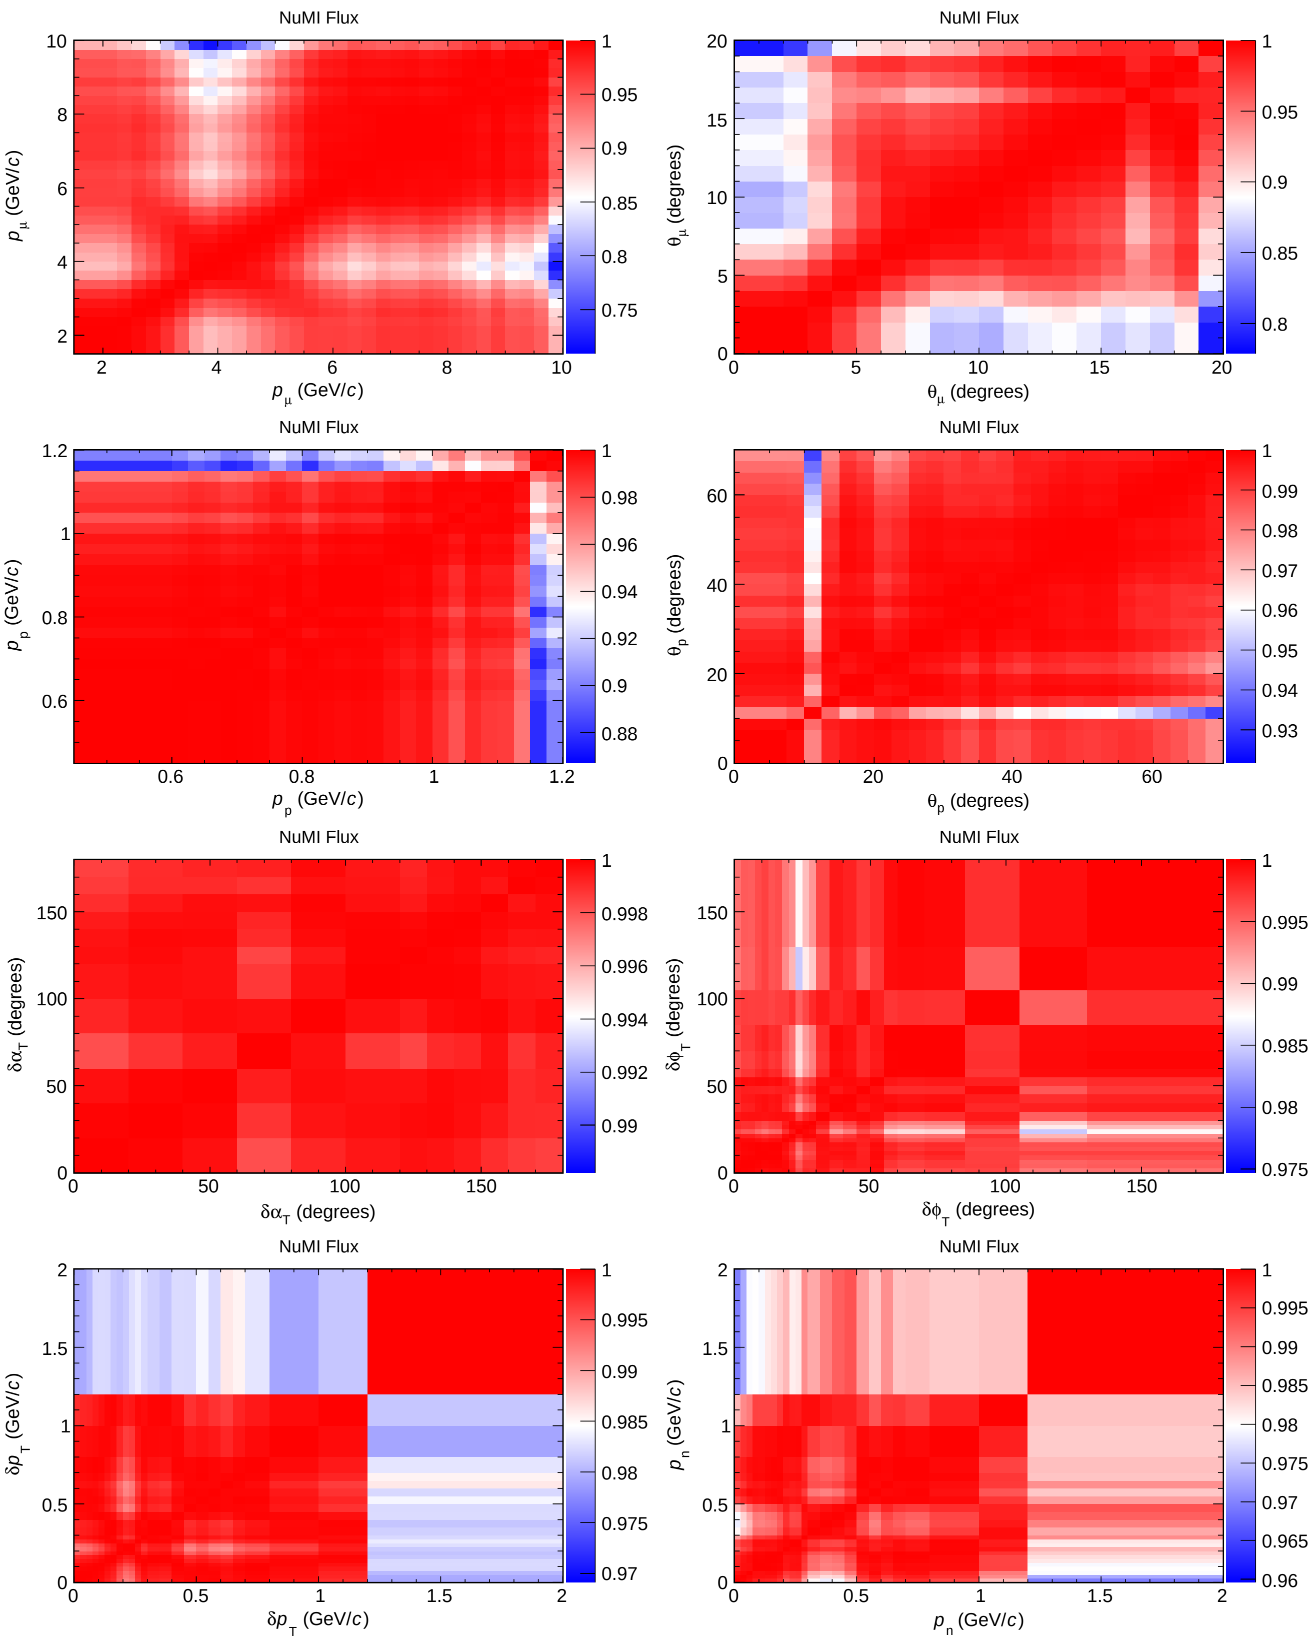


Figure 9: NuMI flux uncertainty correlation matrix for all variables.

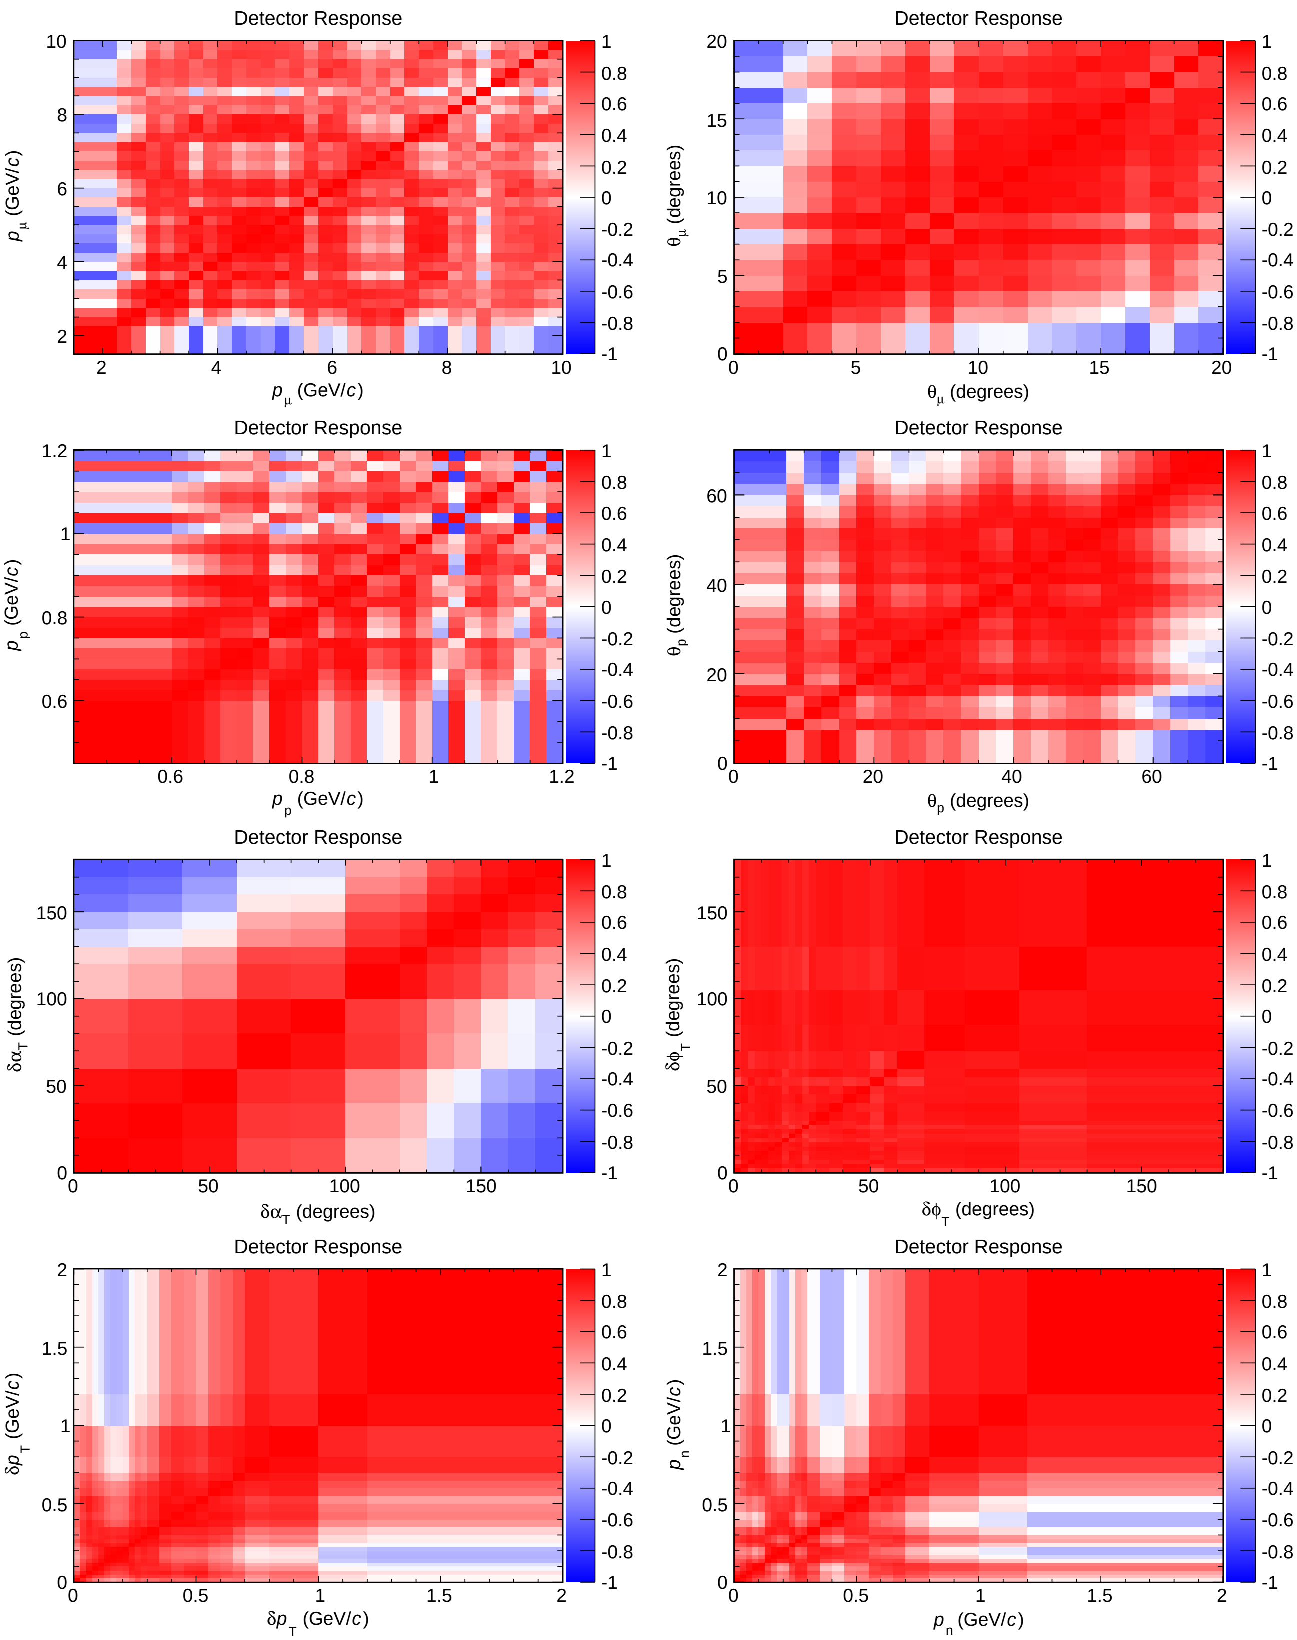


Figure 10: Detector response uncertainty correlation matrix for all variables.

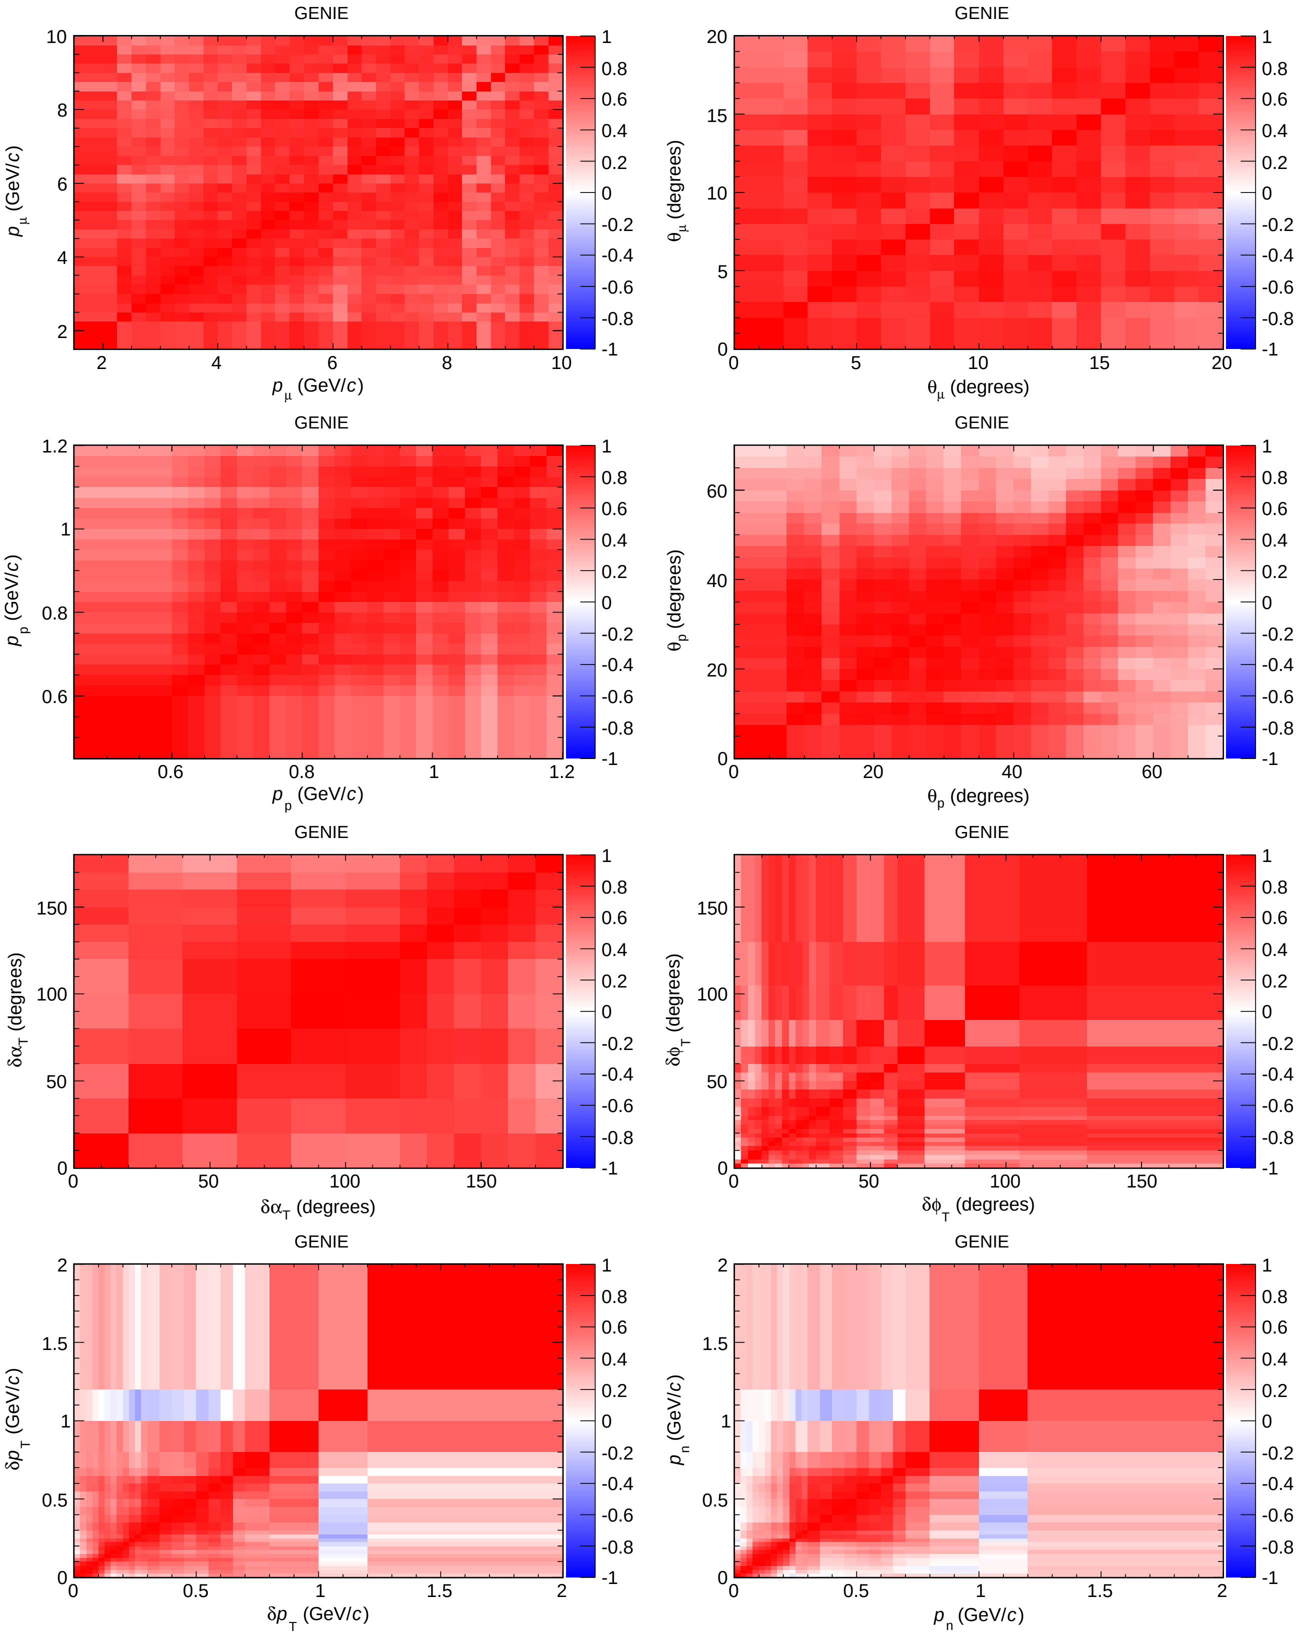


Figure 11: GENIE model uncertainty correlation matrix for all variables.
